# Supplementary material for: The Combinatorial Brain Surgeon: Pruning Weights That Cancel One Another in Neural Networks
Source: arXiv:2203.04466 source file (2022-06-19)
Supplement: Supplementary file 1 [file appendix_exp.tex]

\begin{table}[]
    \centering
    \begin{small}
        \begin{tabular}{lccc}
            \toprule
            Sparsity & \textit{CBS} & \textit{Mag.} & \textit{WoodFisher} \\
            \midrule
            0.1     &93.988$\pm$    &93.99 $\pm$    & 93.99$\pm$      \\
            0.2     &94.002$\pm$    &94.03 $\pm$    & 94.03$\pm$       \\
            0.3     &94.01 $\pm$    &94.01 $\pm$    & 94.01$\pm$       \\
            0.4     &94.002$\pm$    &93.99 $\pm$    & 93.99$\pm$    \\
            0.5     &93.958$\pm$    &93.93 $\pm$    & 93.93$\pm$     \\
            0.6     &93.964$\pm$    &93.78 $\pm$    & 93.78$\pm$     \\
            0.7     &93.978$\pm$    &93.62 $\pm$    & 93.62$\pm$     \\
            0.8     &93.898$\pm$    &92.89 $\pm$    & 92.89$\pm$      \\
            0.9     &93.136$\pm$    &90.3  $\pm$    & 90.3 $\pm$      \\
            0.95    &88.922$\pm$    &83.64$\pm$     & 83.64$\pm$ \\
            0.98    &55.454$\pm$    &32.25$\pm$     & 32.25$\pm$ \\
            \midrule
            Sparsity & \textit{CBS-S} & \textit{Mag.} & \textit{WoodFisher-S} \\
            \midrule
            0.1     &93.994 $\pm$    &93.99 $\pm$    &93.96 $\pm$      \\
            0.2     &94.056 $\pm$    &94.03 $\pm$    &94.08 $\pm$       \\
            0.3     &94.022 $\pm$    &94.01 $\pm$    &94.04 $\pm$       \\
            0.4     &94.014 $\pm$    &93.99 $\pm$    &94.004$\pm$    \\
            0.5     &93.91  $\pm$    &93.93 $\pm$    &93.928$\pm$     \\
            0.6     &93.846 $\pm$    &93.78 $\pm$    &93.748$\pm$     \\
            0.7     &93.746 $\pm$    &93.62 $\pm$    &93.484$\pm$     \\
            0.8     &93.59  $\pm$    &92.89 $\pm$    &93.128$\pm$      \\
            0.9     &92.366 $\pm$    &90.3  $\pm$    &90.766$\pm$      \\
            0.95    &88.242 $\pm$    &83.64$\pm$     &83.162$\pm$ \\
            0.98    &66.642 $\pm$    &32.25$\pm$     &34.55 $\pm$ \\
            \bottomrule
        \end{tabular}
    \end{small}
    \vspace{-0.1in}
    \caption{The pruning performacne of different methods on MLPNet trained on MNIST. The results were averaged over five runs.}
    \label{table:mlpnet.rst}
    \vspace{-0.1in}
\end{table}

\begin{table}[]
    \centering
    \begin{small}
        \begin{tabular}{lcccc}
            \toprule
            Sparsity & \textit{CBS} & \textit{Mag.} & \textit{WoodFisher} \\
            \midrule
            0.1     &79.81 $\pm$    &79.75  $\pm$    &79.75$\pm$      \\
            0.2     &79.806$\pm$    &79.75  $\pm$    &79.75$\pm$       \\
            0.3     &79.804$\pm$    &79.75  $\pm$    &79.75$\pm$       \\
            0.4     &79.796$\pm$    &79.75  $\pm$    &79.75$\pm$    \\
            0.5     &79.822$\pm$    &79.77  $\pm$    &79.76$\pm$     \\
            0.6     &79.852$\pm$    &79.9   $\pm$    &79.77$\pm$     \\
            0.7     &79.722$\pm$    &79.49  $\pm$    &79.65$\pm$     \\
            0.8     &78.582$\pm$    &76.92  $\pm$    &78.72$\pm$      \\
            0.9     &65.524$\pm$    &49.91  $\pm$    &61.95$\pm$      \\
            0.95    &21.072$\pm$    &10.12 $\pm$     &15.29$\pm$ \\
            0.98    &12.162$\pm$    &$\pm$     &9.9$\pm$ \\
            \midrule
            Sparsity & \textit{CBS-S} & \textit{Mag.} & \textit{WoodFisher-S} \\
            \midrule
            0.1     &79.794 $\pm$    &79.75  $\pm$    &79.75$\pm$      \\
            0.2     &79.794 $\pm$    &79.75  $\pm$    &79.75$\pm$       \\
            0.3     &79.784 $\pm$    &79.75  $\pm$    &79.75$\pm$       \\
            0.4     &79.79  $\pm$    &79.75  $\pm$    &79.75$\pm$    \\
            0.5     &79.836 $\pm$    &79.77  $\pm$    &79.76$\pm$     \\
            0.6     &79.856 $\pm$    &79.9   $\pm$    &79.87$\pm$     \\
            0.7     &79.472 $\pm$    &79.49  $\pm$    &79.78$\pm$     \\
            0.8     &77.822 $\pm$    &76.92  $\pm$    &77.24$\pm$      \\
            0.9     &62.092 $\pm$    &49.91  $\pm$    &52.66$\pm$      \\
            0.95    &32.632 $\pm$    &10.12 $\pm$     &14.81$\pm$ \\
            0.98    &15.494 $\pm$    &      $\pm$     &9.34 $\pm$ \\
            \bottomrule
        \end{tabular}
    \end{small}
    \vspace{-0.1in}
    \caption{The pruning performacne of different methods on CifarNet trained on Cifar10. The results were averaged over five runs.}
    \label{table:cifarnet.rst}
    \vspace{-0.1in}
\end{table}

\begin{table}[]
    \centering
    \begin{small}
        \begin{tabular}{lccc}
            \toprule
            Sparsity & \textit{CBS} & \textit{Mag.} & \textit{WoodFisher} \\
            \midrule
            %0.1     &93.988$\pm$    &93.99 $\pm$    & 93.99$\pm$      \\
            %0.2     &94.002$\pm$    &94.03 $\pm$    & 94.03$\pm$       \\
            %0.3     &94.01 $\pm$    &94.01 $\pm$    & 94.01$\pm$       \\
            %0.4     &94.002$\pm$    &93.99 $\pm$    & 93.99$\pm$    \\
            0.5     &93.958$\pm$    &93.93 $\pm$    & 93.93$\pm$     \\
            %0.6     &93.964$\pm$    &93.78 $\pm$    & 93.78$\pm$     \\
            0.7     &93.978$\pm$    &93.62 $\pm$    & 93.62$\pm$     \\
            %0.8     &93.898$\pm$    &92.89 $\pm$    & 92.89$\pm$      \\
            0.9     &93.136$\pm$    &90.3  $\pm$    & 90.3 $\pm$      \\
            0.95    &88.922$\pm$    &83.64$\pm$     & 83.64$\pm$ \\
            0.98    &55.454$\pm$    &32.25$\pm$     & 32.25$\pm$ \\
            \midrule
            Sparsity & \textit{CBS-S} & \textit{Mag.} & \textit{WoodFisher-S} \\
            \midrule
            %0.1     &93.994 $\pm$    &93.99 $\pm$    &93.96 $\pm$      \\
            %0.2     &94.056 $\pm$    &94.03 $\pm$    &94.08 $\pm$       \\
            %0.3     &94.022 $\pm$    &94.01 $\pm$    &94.04 $\pm$       \\
            %0.4     &94.014 $\pm$    &93.99 $\pm$    &94.004$\pm$    \\
            0.5     &93.91  $\pm$    &93.93 $\pm$    &93.928$\pm$     \\
            %0.6     &93.846 $\pm$    &93.78 $\pm$    &93.748$\pm$     \\
            0.7     &93.746 $\pm$    &93.62 $\pm$    &93.484$\pm$     \\
            %0.8     &93.59  $\pm$    &92.89 $\pm$    &93.128$\pm$      \\
            0.9     &92.366 $\pm$    &90.3  $\pm$    &90.766$\pm$      \\
            0.95    &88.242 $\pm$    &83.64$\pm$     &83.162$\pm$ \\
            0.98    &66.642 $\pm$    &32.25$\pm$     &34.55 $\pm$ \\
            \bottomrule
        \end{tabular}
    \end{small}
    \vspace{-0.1in}
    \caption{The pruning performance (Top1 accuracy) of different methods on MLPNet trained on Cifar10. The accuracy of the model before pruning is 93.97\%. The results were averaged over five runs.}
    \label{table:mlpnet.rst}
    \vspace{-0.1in}
\end{table}

\begin{table}[]
    \centering
    \begin{small}
        \begin{tabular}{lcccc}
            \toprule
            Sparsity & \textit{CBS} & \textit{Mag.} & \textit{WoodFisher} \\
            \midrule
            %0.1     &79.81 $\pm$    &79.75  $\pm$    &79.75$\pm$      \\
            %0.2     &79.806$\pm$    &79.75  $\pm$    &79.75$\pm$       \\
            %0.3     &79.804$\pm$    &79.75  $\pm$    &79.75$\pm$       \\
            %0.4     &79.796$\pm$    &79.75  $\pm$    &79.75$\pm$    \\
            %0.5     &79.822$\pm$    &79.77  $\pm$    &79.76$\pm$     \\
            %0.6     &79.852$\pm$    &79.9   $\pm$    &79.77$\pm$     \\
            0.7     &79.722$\pm$    &79.49  $\pm$    &79.65$\pm$     \\
            0.8     &78.582$\pm$    &76.92  $\pm$    &78.72$\pm$      \\
            0.9     &65.524$\pm$    &49.91  $\pm$    &61.95$\pm$      \\
            0.95    &21.072$\pm$    &10.12 $\pm$     &15.29$\pm$ \\
            0.98    &12.162$\pm$    &$\pm$     &9.9$\pm$ \\
            \midrule
            Sparsity & \textit{CBS-S} & \textit{Mag.} & \textit{WoodFisher-S} \\
            \midrule
            %0.1     &79.794 $\pm$    &79.75  $\pm$    &79.75$\pm$      \\
            %0.2     &79.794 $\pm$    &79.75  $\pm$    &79.75$\pm$       \\
            %0.3     &79.784 $\pm$    &79.75  $\pm$    &79.75$\pm$       \\
            %0.4     &79.79  $\pm$    &79.75  $\pm$    &79.75$\pm$    \\
            %0.5     &79.836 $\pm$    &79.77  $\pm$    &79.76$\pm$     \\
            %0.6     &79.856 $\pm$    &79.9   $\pm$    &79.87$\pm$     \\
            0.7     &79.472 $\pm$    &79.49  $\pm$    &79.78$\pm$     \\
            0.8     &77.822 $\pm$    &76.92  $\pm$    &77.24$\pm$      \\
            0.9     &62.092 $\pm$    &49.91  $\pm$    &52.66$\pm$      \\
            0.95    &32.632 $\pm$    &10.12 $\pm$     &14.81$\pm$ \\
            0.98    &15.494 $\pm$    &      $\pm$     &9.34 $\pm$ \\
            \bottomrule
        \end{tabular}
    \end{small}
    \vspace{-0.1in}
    \caption{The pruning performance (Top-1 test acc.) of different methods on CifarNet trained on Cifar10. The accuracy of the model before pruning is 79.75\%. The results were averaged over five runs.}
    \label{table:cifarnet.rst}
    \vspace{-0.1in}
\end{table}

\begin{table}[]
    \centering
    \begin{small}
        \begin{tabular}{lcccc}
            \toprule
            Sparsity & \textit{CBS} & \textit{Mag.} & \textit{WoodFisher} \\
            \midrule
%0.1     &91.388 &91.43  &91.366 \\
%0.2     &91.368 &91.39  &91.338 \\
%0.3     &91.352 &90.77  &91.366 \\
0.4     &91.206 &89.98  &91.152 \\
%0.5     &90.578 &88.44  &90.233 \\
0.6     &88.88  &85.24  &87.958 \\
0.7     &81.838 &78.79  &81.046 \\
0.8     &51.278 &54.01  &62.632 \\
0.9     &13.676 &11.79  &11.488 \\
            \midrule
            Sparsity & \textit{CBS-S} & \textit{Mag.} & \textit{WoodFisher-S} \\
            \midrule
%0.1     &91.402 &91.43  &91.444 \\
%0.2     &91.308 &91.39  &91.368 \\
%0.3     &90.97  &90.77  &90.814 \\
0.4     &90.656 &89.98  &90.02  \\
%0.5     &89.32  &88.44  &88.062 \\
0.6     &86.482 &85.24  &84.946 \\
0.7     &79.554 &78.79  &78.092 \\
0.8     &61.3   &54.01  &52.054 \\
0.9     &16.834 &11.79  &11.442 \\
            \bottomrule
        \end{tabular}
    \end{small}
    \vspace{-0.1in}
    \caption{The pruning performance of different methods on ResNet20 trained on Cifar10. The unpruned model has top-1 accuracy of 91.36\%. The results were averaged over five runs.}
    \label{table:resnet20.rst}
    \vspace{-0.1in}
\end{table}

\begin{table}[]
    \centering
    \begin{small}
        \begin{tabular}{lcccc}
            \toprule
            Sparsity & \textit{Mag.} & \textit{Mag. + CBS-U} & \textit{WF(S+U)} & \textit{WF-S + CBS-U} \\
            \midrule
0.2&    72.046& 71.994  &72.014 &71.998 \\
0.3&    71.606& 71.878  &71.876 &71.862 \\
0.4&    69.158& 71.43   &71.152 &71.432 \\
0.5&    62.61 &  70.244 &68.908 &70.3   \\
0.6&    41.94 &  66.328 &60.896 &66.616 \\
0.7&    6.784 &  55.512 &29.36  &56.088 \\
0.8&    0.108 &  16.584 &0.24   &17.936 \\
0.9&    TBD   &  0.12   &0.1    &0.11 \\

            \bottomrule
        \end{tabular}
    \end{small}
    \vspace{-0.1in}
    \caption{Ablation study on CBS-U and comparision with the weight update of WoodFisher method. This is tested on MobileNet trained on ImageNet with the accuracy of 72.0\% before pruning.}
    \label{table:ablation.update}
    \vspace{-0.1in}
\end{table}
